# Supplementary material for: Erasable superconductivity in topological insulator Bi2Se3 induced by voltage pulse
Source: arXiv:2106.13207 source file (2021-06-24)
Supplement: Supplementary file 1 [file Supporting_information.pdf]

# Supporting Information

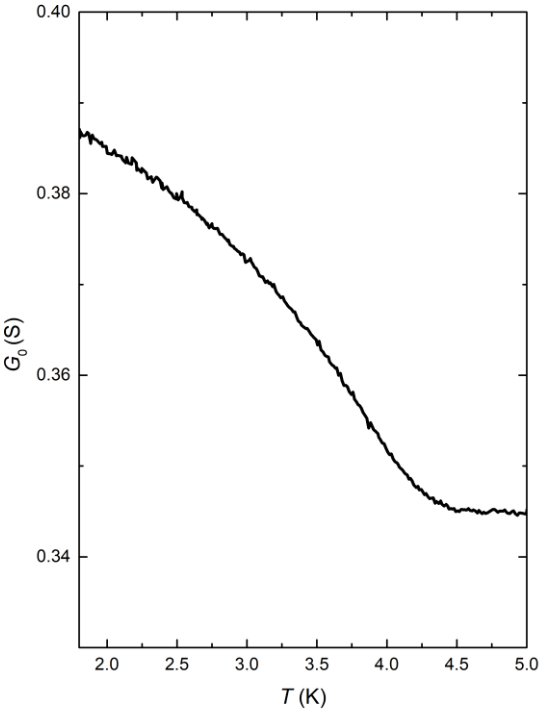


**Fig. S1** Temperature dependence of zero bias conductance (ZBC) for the soft-PCS on $Bi_2Se_3$.

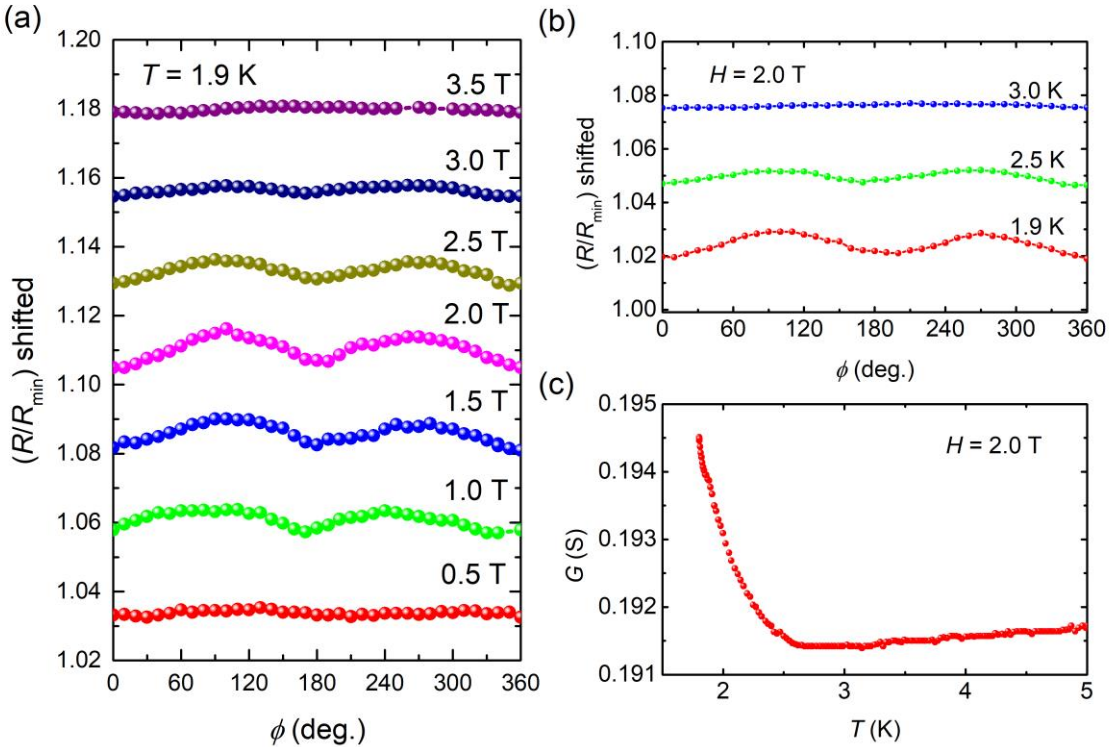


**Fig. S2** (a) Angle dependence of ZBR for the soft-PCS at different magnetic fields within the ab-plane at 1.9 K; (b) Angle dependence of ZBR for the soft-PCS at different temperatures within the

ab-plane at 2.0 T; (c) Temperature dependence of ZBR for the soft-PCS on $Bi_2Se_3$ at 2.0 T;

## 1. Analysis on the width of ZBCP

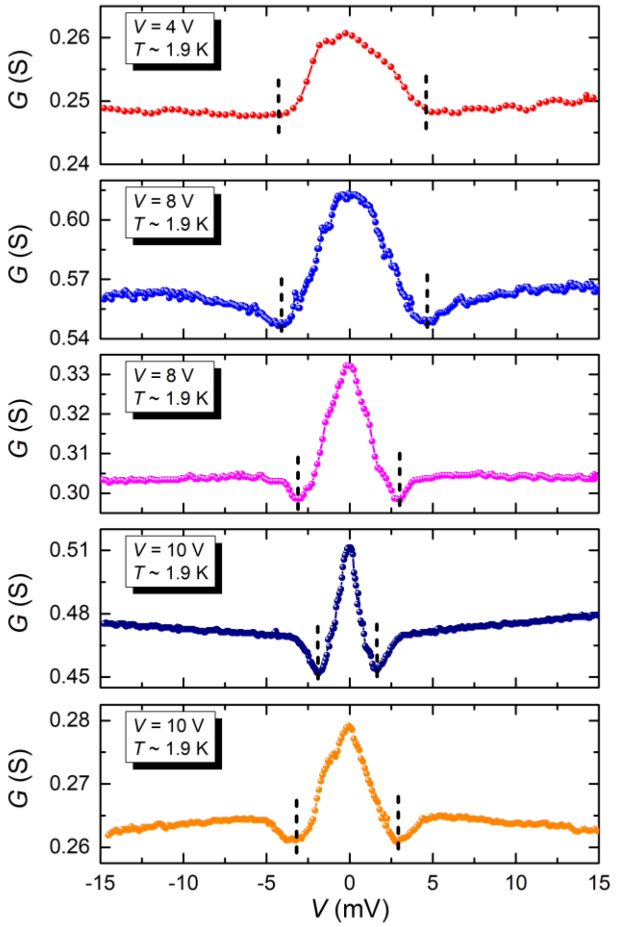


**Fig. S3** The different width of ZBCP for Ag-$Bi_2Se_3$ contacts with different intensity of voltage pulse.

The width of the ZBCP is related to the superconductor gap order parameter as well as superconducting transition temperature $T_c$. When charged with different magnitude of voltage pulse, the width of ZBCP and $T_c$ can be different. Moreover, we note that the ZBCP width can also be influenced by the detailed contact condition such as contact area and resistance. It sometimes can be arbitrary: The voltage with 4 V can induce a wider ZBCP than 10 V and the width of ZBCP can be different even for the same voltage as shown in Fig. S3. According to the proposed Ag atoms injection scenario, the Ag atoms are injected into vdW gap by voltage pulse and can also escape from the vdW gap due to locally raised temperature by heating effect from the high voltage. After going through different thermal cycles, the width and height of ZBCP

will decrease as evidenced by Fig. 2(d) in the main text.

## 2. Exclusion of local strain, structural changes or impurity phase

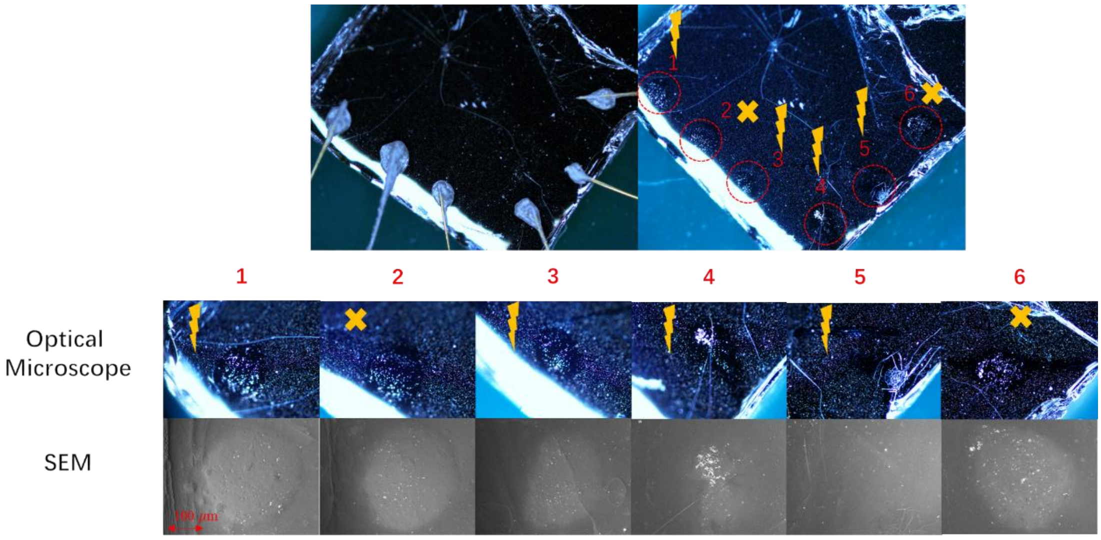


Fig. S4 Optical and SEM images of the soft point contacts with silver paints after the measurements.

We have conducted a comparative study with optical microscope and SEM to check whether the sample has been damaged after voltage pulses: As in Fig. S4, the contacts 1, 3, 4, 5 were treated with voltage pulses and superconductivity was locally induced, while the contacts 2, 6 are pristine without the application of voltage pulses. The two categories of contacts do not show any noticeable difference between them except some residual silver particles, confirming that the sample has not been damaged. Meanwhile, it is difficult for us to characterize the local structural changes by AFM or STM because the sample surface is not fresh anymore after soft point-contacts and the exact contact positions in mechanical point-contacts can't be marked during the experiments.

However, if the superconductivity is induced by local strain or structural changes, it is hard to explain the fact that superconductivity only appears in Ag-$Bi_2Se_3$ contacts. In contrast, we should observe the similar effect in Au-, Ti- and Cu-$Bi_2Se_3$ contacts, but it is not the case. We can thus exclude the scenario of local strain and structural changes. As for other impurity phase, the possible compounds with Ag, Bi or Se elements include $Ag_3Bi$, $Ag_2Se$ and $Ag_xBi_{2-x}Se_3$. The superconductivity behavior in $Ag_3Bi$ and $Ag_2Se$

have not been reported yet. In $Ag_xBi_{2-x}Se_3$, the partial Bi atoms are replaced by Ag and superconductivity is only reported at high pressures above 11GPa (*PRB 97, 104503 (2018)*). In conclusion, we proposed that the injection of Ag atoms into vdW gap by voltage pulse should result in the superconductivity in our Ag-$Bi_2Se_3$ contacts. We note that superconductivity in $Ag_xBi_2Se_3$ has also been predicted in a recent theoretical paper (*arXiv:1904.03698 (2019)*).
